# Supplementary material for: SoftMatcha: A Soft and Fast Pattern Matcher for Billion-Scale Corpus Searches
Source: arXiv:2503.03703 source file (2025-03-05)
Supplement: Supplementary file 1 [file gloss.tex]

\section{Glossing for Latin}\label{sec:gloss}
The interlinear glossing texts for the Latin sentences used in this paper are shown below.

\pex
\a \begingl
    \glpreamble Query: \textit{factus est} //
    \gla factus est //
    \glb do.\textsc{pass.pf.ptcp.m.sg} be.\textsc{ind.prs.3sg} //
    \glft `(he/she/it) is done' //
\endgl
\a \begingl
    \gla facta sunt //
    \glb do.\textsc{pass.pf.ptcp.n.pl} be.\textsc{ind.prs.3pl} //
    \glft `they are done' or `they are facts' //
\endgl
\a \begingl
    \gla mortuus esset //
    \glb die.\textsc{act.pf.ptcp.m.sg} be.\textsc{sub.impf.3sg} //
    \glft `(that he/she/it) was dead' //
\endgl
\a \begingl
    \gla creatus erat //
    \glb create.\textsc{pass.pf.ptcp.m.sg} be.\textsc{ind.impf.3sg} //
    \glft `(he/she/if) was created' //
\endgl
\xe

\pex
\a
    \begingl
        \glpreamble Query: \textit{non possum} //
        \gla non possum //
        \glb not can.\textsc{ind.prs.1sg} //
        \glft `I cannot' //
    \endgl
\a
    \begingl
        \gla non potero //
        \glb not can.\textsc{ind.fut.1sg} //
        \glft `I will not be able to' //
    \endgl
\a
    \begingl
        \gla non nolim //
        \glb not not.want.\textsc{sub.prs.1sg} //
        \glft `not that I would not like to' //
    \endgl
\xe

\pex
\a
    \begingl
        \glpreamble Query: \textit{equus est} //
        \gla equus est //
        \glb horse.\textsc{m.nom.sg} be.\textsc{ind.prs.3sg} //
        \glft `(he/she/it) is a horse' //
    \endgl
\a
    \begingl
        \gla bos est //
        \glb cow.\textsc{f.nom.sg} be.\textsc{ind.prs.3sg} //
        \glft `(he/she/it) is a cow' //
    \endgl
\a
    \begingl
        \gla Minotaurus esset //
        \glb Minotaur.\textsc{m.nom.sg} be.\textsc{sub.impf.3sg} //
        \glft `(he/she/it) was the Minotaur' //
    \endgl
\xe

\pex
\a
    \begingl
        \glpreamble Query: \textit{bellum Gallicum} (book by Julius Caesar) //
        \gla bellum Gallicum //
        \glb war.\textsc{n.nom.sg} Gallic.\textsc{n.nom.sg} //
        \glft `the Gallic war' //
    \endgl
\a
    \begingl
        \gla bellum Etruscum //
        \glb war.\textsc{n.nom.sg} Etruscan.\textsc{n.nom.sg} //
        \glft `the Etrucan war' //
    \endgl
\a
    \begingl
        \gla contra Caesarem //
        \glb against Caesar.\textsc{m.acc.sg} //
        \glft `against Caesar'//
    \endgl
\xe

\pex
\a
    \begingl
        \glpreamble Query: \textit{quo vadis} (Bible, John 13:36) //
        \gla quo vadis //
        \glb where go.\textsc{ind.prs.2sg} //
        \glft `where do you go?' //
    \endgl
\a
    \begingl
        \gla ibi vadis //
        \glb there go.\textsc{ind.prs.2sg} //
        \glft `you go there' //
    \endgl
\a\label{ex:augustine}
    \begingl
        \gla
        % Si autem tu potius in errore atque in impietate versaris % comment out this line for a shorter version
        % ..., quo 
        autem voc\=aris
        % ibi est veritas et pietas, ...
        % quia ibi Christiana unitas et sancti spiritus caritas, quid adhuc tibi esse conaris inimicus? % comment out this line for a shorter version
        //
        \glb
        % if but you.\textsc{nom.sg} rather in error.\textsc{m.sg.abl} and in impiety.\textsc{f.sg.abl} stay.\textsc{act.ind.prs.2sg} % comment out this line for a shorter version
        % ~ in.which
        but summon.\textsc{pass.ind.prs.2sg}
        % there be.\textsc{ind.prs.3sg} truth.\textsc{f.nom.sg} and charity.\textsc{f.nom.sg} 
        % because there Christian.\textsc{f.nom.sg} unity.\textsc{f.nom.sg} and holy.\textsc{m.gen.sg} spirit.\textsc{m.gen.sg} charity.\textsc{f.nom.sg} why still you.\textsc{dat.sg} be.\textsc{inf.prs} try.\textsc{act.ind.prs.2sg} enemy.\textsc{m.nom.sg} % comment out this line for a shorter version
        //
        \glft 
        % But if you rather are living in error and in impiety, and truth and piety rather exist % comment out this line for a shorter version
        % but truth and piety rather exist 
        `but you are summoned'
        % for the reason that there are to be found Christian unity and the charity of the Holy Spirit, why do you keep on trying to be your own worst enemy?' % comment out this line for a shorter version
        //
    \endgl
\xe

\pex
\a
    \begingl
        \glpreamble Query: quod erat demonstrandum (Q.E.D.) //
        \gla quod erat demonstrandum //
        \glb which.\textsc{n.nom.sg} be.\textsc{ind.impf.3sg} demonstrate.\textsc{pass.fut.ptcp.n.sg} //
        \glft `which was to be shown' //
    \endgl
\a
    \begingl
        \gla haec erat forma //
        \glb this.\textsc{f.nom.sg} be.\textsc{ind.impf.3sg} form.\textsc{f.nom.sg} //
        \glft `this was the form' //
    \endgl
\a
    \begingl
        \gla quod postea accipiamus //
        \glb which.\textsc{n.nom.sg} afterwards accept.\textsc{act.sub.prs.1pl} //
        \glft `which we shall accept afterwards' //
    \endgl
\xe
